# Supplementary material for: Nematic order from phase synchronization of shape oscillations
Source: arXiv:2503.04282 ancillary file (2025-07-09)
Supplement: Supplementary file 1 [file Supplemental_Material.pdf]

# Supplemental Material for “Nematic order from phase synchronization of shape oscillations”

Ioannis Hadjifrangiskou[1], Sumesh Thampi[1], and Rahil N. Valani[1]*
[1] *Rudolf Peierls Centre for Theoretical Physics, Parks Road, University of Oxford, OX1 3PU, United Kingdom*
(Dated: March 5, 2025)

## I. ADDITIONAL RESULTS FOR PHASE SYNCHRONIZATION OF DEFORMABLE PARTICLES

In addition to the results presented in the main text for deformable particles in planar shear flow (Eqs. (1)-(3) of the main text) with shear rate $\dot{\gamma}(t) = 1 + A\sin(\omega t)$, we provide additional results in this section related to the phase synchronization dynamics.

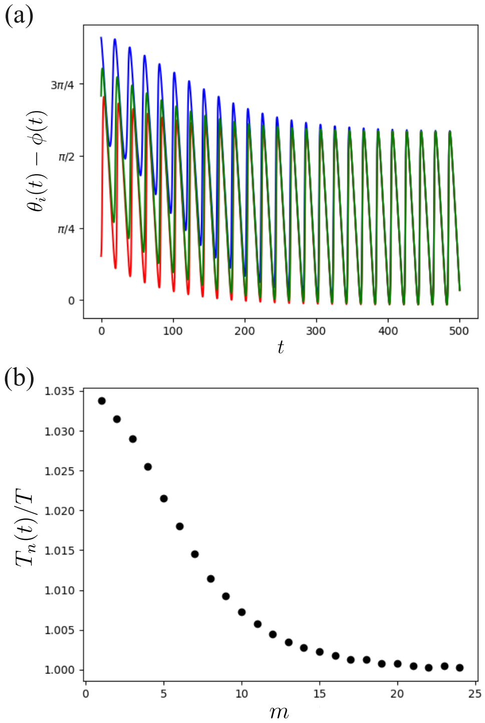


FIG. 1. Phase locking and frequency locking during synchronization for the parameter values in Fig. 1 of the main text. (a) Phase difference between the driven oscillator of each particle and the driving oscillator, $\theta_i(t) - \phi(t)$, with $\phi(t) = \omega t$, as a function of time for three different initial conditions (red, blue, green). (b) Evolution of the time period of the limit cycle $T_n(t)$ scaled with the driving period $T$ as a function of the number of driving periods $m$. The time period was calculated as the duration between consecutive peaks in the time series of $\theta_i(t)$.

* rahil.valani@physics.ox.ac.uk

### A. Phase and frequency locking

The phase synchronization mechanism present in the main text results in phase and frequency locking of particles' shape and orientation oscillations to the oscillatory component of the shear flow. This phase and frequency locking is shown in Fig. 1(a) and (b), respectively. For phase locking, we see that the difference between the phase of each particle's orientation and driving, i.e. $\theta_i(t) - \phi(t)$ with $\phi(t) = \omega t$, stays bounded and converges on a unique oscillatory behavior for different particles, i.e. initial conditions (see Fig. 1(a)). This is consistent with the general definition of phase locking where the differences between the phases should be bounded and the difference does not necessarily need to be zero or a constant value [1]. Further, from Fig. 1(b), we see that the period of the orientational oscillations converges to the period of driving $T$ with time resulting in frequency locking.

### B. Saddle-node bifurcation of cycles and Arnold Tongues

The appearance and disappearance of synchronized regions as Arnold tongues in the parameter space formed by $T/T_n$ and $A$ (see Fig. 3(a) of the main text and also Fig. 2(a)) is due to saddle-node bifurcation of limit cycles in state space. If we fix $A = 0.5$ and traverse horizontally in the parameter-space towards larger $T$ (with $T_n \approx 20.02$ ) near the first tongue, then at the onset of the synchronization region, a pair of stable and unstable (saddle) limit cycles are born that appear as a stable (cyan circle) and an unstable (pink cross) point in the 2D polar $(r, 2\theta)$ section of the state-space shown in Fig. 2(b) for $T = 19.5$. Increasing $T$ inside the first synchronization tongue results in the pair of stable and unstable points moving away from each other along the limit cycle (red) of the non-oscillatory ($A = 0$) system (see Fig. 2(b)-(c)). At even larger $T$ as one approaches the other end of the tongue, the two fixed points approach each other again on the limit cycle, as shown in Fig. 2(d) for $T = 20.78$, and annihilate each other via a saddle-node bifurcation of cycles. Thus, the periodic appearances of synchronization tongues near multiples of the natural period of the limit cycle $T_n$ are facilitated by these saddle-node bifurcations of limit cycles.

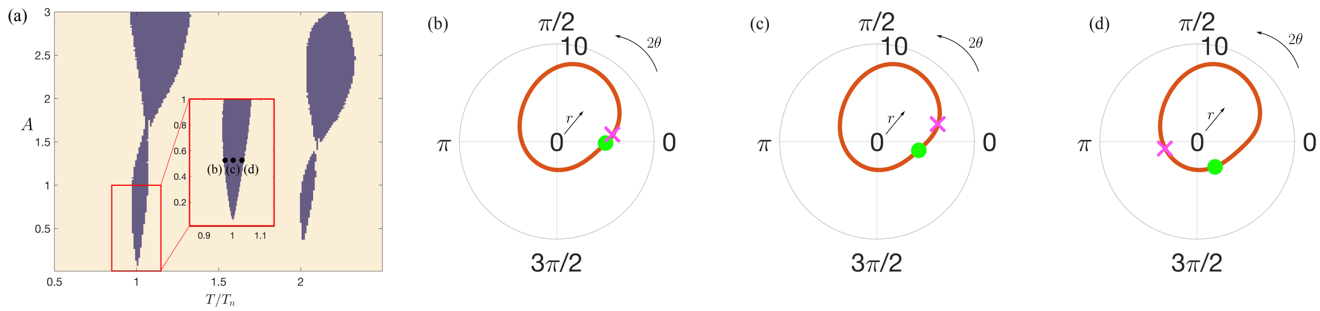


FIG. 2. (a) Regions of phase-synchronization-induced nematic order (violet) in the $(T/T_n, A)$. Arnold tongues that are characteristic of synchronization, are observed at multiples of the natural period of the limit cycle $T_n \approx 20.02$. Two-dimensional $(r, 2\theta)$ section of the state-space showing (b) the birth of stable (cyan circle) and an unstable (pink cross) points via a saddle-node bifurcation on the limit cycle (red) of the non-oscillatory system ($A = 0$) near $T = 19.5$. (c) These fixed points spread on the limit cycle near the middle of the tongue ($T = 20$) and (d) then annihilate again in a saddle-node bifurcation at the other end of the tongue ($T = 20.78$).

### C. Time taken to synchronize based on initial conditions

Although we achieve phase synchronization for all particles, i.e. all different initial conditions, as $t \to \infty$ in the synchronization regions of the parameter space, the amount of time it takes to phase synchronize can vary depending on the initial conditions. This is because, phase synchronization in state space corresponds to converging onto the stable limit cycle where another unstable (saddle) limit cycle also exists. Hence, if an initial condition in state space is near a stable limit cycle, then it can quickly converge onto this cycle. Conversely, an initial condition near the unstable limit cycle may take a long time to converge onto the stable limit cycle. This contrast in the time taken to converge onto the stable limit cycle is depicted in Fig. 3 where we have plotted the number of driving periods (colormap) required to phase-synchronize based on different initial conditions $\theta(0)$ and $\phi(0)$ for a fixed $r(0) = r_0 = 5$. It can be seen that the convergence is quicker along black regions that correspond to initial conditions that can quickly approach the stable limit cycle. Conversely, convergence is slower along white regions that correspond to initial conditions that are likely to be in the vicinity of the unstable limit cycle. Thus, the slow development of the nematic order in phase-synchronized regions, as shown in Fig. 1(e) of the main text, can be attributed to initial conditions that start near the unstable limit cycle in state space and take a long time to converge onto the stable limit cycle.

### D. Synchronization of deformable particles in time-dependent shear flow with large oscillatory component

In the main text, we mainly focused on phase synchronization in the regime where $A < 1$. However, even for $A > 1$, we find that synchronized regions persist and interestingly, we obtain time-periodic states that undergo a more complex oscillation mode in the synchronized phase with a mixture of tumbling and back-and-forth oscillations. An example is shown in Fig. 4 where kymograph of orientation $\theta_i(t)$ and shape parameter $r_i(t)$ for $N = 50$ particles are shown at early and late times in panel (a) and (b), respectively. We find that for the parameter values corresponding to Fig. 4, we obtain a mixed mode composed of one tumbling and one back-and-forth orientational oscillation (see Supplemental Video S4).

### E. Synchronization of deformable particles in oscillating shear flow with no mean flow

We also find phase synchronization in completely oscillatory shear flow without any mean flow component i.e. $\dot{\gamma}(t) = A\sin(\omega t)$. An example with kymographs is shown in Fig. 5 for $A = 1$ and $T = 20$. Here, instead of the particle undergoing any tumbling motion, we find a pure back-and-forth orientational oscillations which are synchronized to the driving oscillating shear (see also Supplemental Video S5).

## II. MATHEMATICAL ANALYSIS OF SYNCHRONIZATION FOR DEFORMABLE AND RIGID PARTICLES

Consider a general dynamical system of the form

$$\dot{\mathbf{x}} = F(\mathbf{x}; \alpha),$$

where $\mathbf{x}$ is the vector consisting of all the dynamical variables, $F(\cdot)$ is a general nonlinear differentiable function and $\alpha$ is a control parameter of the system. If we now allow this control parameter to oscillate in time with some small amplitude $\epsilon$, i.e. $\alpha(t) = \alpha_0 + \epsilon\sin(\omega t)$, then we have

$$\dot{\mathbf{x}} = F(\mathbf{x}; \alpha_0 + \epsilon\sin(\omega t)).$$

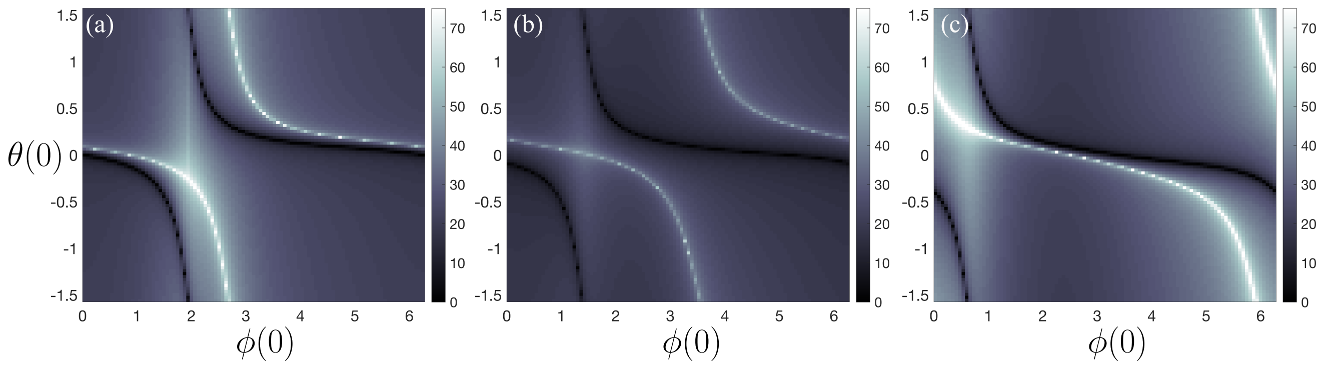


FIG. 3. Time taken for phase synchronization based on initial conditions $\phi(0)$ and $\theta(0)$ for the system of deformable particles presented in Fig. 1 the main text. Plots are shown for $A = 0.5$, $r(0) = r_0 = 5$ with (a) $T = 19.5$, (b) $T = 20$ and (c) $T = 20.7$.

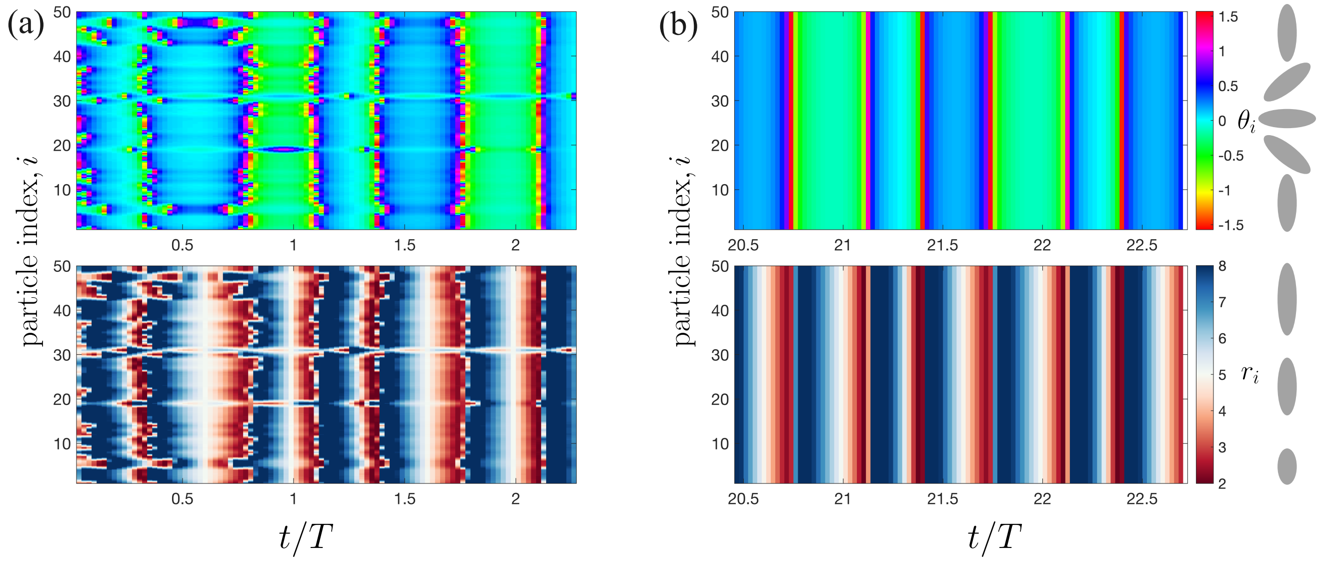


FIG. 4. Phase synchronization of deformable particles in time-dependent shear flow where the oscillatory flow component is larger in magnitude compared to the steady flow component i.e. $\dot{\gamma}(t) = 1 + A\sin(\omega t)$ with $\omega = 2\pi/T$ and $A > 1$. We use the parameters as $A = 3$ and $T = 22$ with $N = 50$ different initial conditions. Plots show evolution at (a) early times and (b) late times of orientation $\theta_i$ (top) and shape parameter $r_i$ (bottom) for each independent particle (i.e. each initial condition). Other parameters are same as Fig. 1 of the main text. See also Supplemental Video S4.

If $\epsilon \ll \alpha_0$, then one can do a perturbation expansion in powers of $\epsilon$ and get the following leading order equations:

$$\dot{\mathbf{x}} \approx F(\mathbf{x}; \alpha_0) + \epsilon \frac{\partial F}{\partial \alpha}\Big|_{\alpha=\alpha_0} \sin(\omega t).$$

Hence, an oscillatory parameter perturbation can be viewed as a periodically varying external driving (with a state dependent coefficient) and we get the general form of the dynamical system as per below

$$\dot{\mathbf{x}} = F(\mathbf{x}; \alpha_0) + \epsilon G(\mathbf{x}; \alpha_0) \sin(\omega t),$$

where

$$G(\mathbf{x}; \alpha_0) = \frac{\partial F}{\partial \alpha}\Big|_{\alpha=\alpha_0}.$$

We now analyze the nonlinear ordinary differential equations (ODEs) that arise in our setup of both, deformable and rigid, elongated particles interacting with time-dependent shear flow in the limit of small-amplitude driving. The reduced equations obtained in this limit, along with the mathematical theory of synchronization, can guide us in identifying systems that exhibit phase synchronization [1, 2].

### A. Deformable particles

We start by considering the case of deformable elongated particle as discussed in the main text. For deformable particles in time-dependent shear flow as presented in the main text, we have the following coupled nonlinear ODEs for the evolution of orientation angle $\theta$

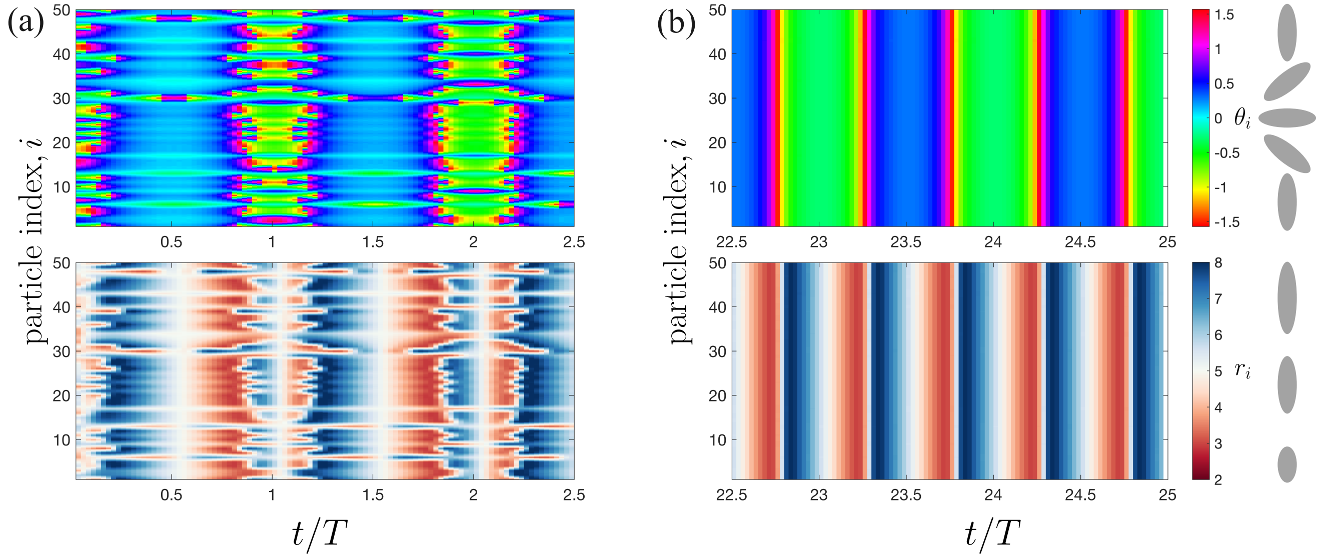


FIG. 5. Phase synchronization of deformable particles in an oscillating shear flow with no mean flow i.e. $\dot{\gamma}(t) = A\sin(\omega t)$ with $\omega = 2\pi/T$. We use the parameters as $A = 1$ and $T = 20$ for no mean flow and $N = 50$ different initial conditions. Plots show evolution at (a) early times and (b) late times of orientation $\theta_i$ (top) and shape parameter $r_i$ (bottom) for each independent particle (i.e. each initial condition). Other parameters are same as Fig. 1 of the main text. See also Supplemental Video S5.

and the shape parameter $r$,

$$\dot{\theta} = \frac{\dot{\gamma}}{2}\left(\frac{(r+1)^2-1}{(r+1)^2+1}\cos 2\theta - 1\right) = F_1(\theta, r; \dot{\gamma}), \tag{1}$$

$$\dot{r} = \dot{\gamma}(r+1)\sin 2\theta - \frac{1}{\alpha}(r-r_0)\left(1+\epsilon(r-r_0)^2\right) \tag{2}$$
$$= F_2(\theta, r; \dot{\gamma}).$$

As described in the main text, the parameters $\alpha$ and $\epsilon$ are related to the free energy of the shape parameter $r$ that maintains an equilibrium shape parameter of $r_0$ in the absence of flow. Keeping other parameters fixed, we are mainly interested in the parameter $\dot{\gamma}$ that will vary as a function of time in a time-dependent shear flow. Rewriting the system in vector notation we have

$$\dot{\mathbf{x}} = F(\mathbf{x}; \dot{\gamma}),$$

where $\mathbf{x} = (\theta, r)$ and $F(\mathbf{x}; \dot{\gamma}) = (F_1(\theta, r; \dot{\gamma}), F_2(\theta, r; \dot{\gamma}))$. If we now let $\dot{\gamma}(t) = 1 + A\sin(\omega t)$ then we can do a perturbation expansion in $A$ assuming $A \ll 1$, and we get the following leading order equation

$$\dot{\mathbf{x}} \approx F(\mathbf{x}) + A\,G(\mathbf{x})\sin(\omega t).$$

Here, $F(\mathbf{x}) = F(\mathbf{x}; \dot{\gamma})\big|_{\dot{\gamma}=1}$ and

$$G(\mathbf{x}) = (G_1, G_2) = \left(\frac{\partial F_1(\mathbf{x}; \dot{\gamma})}{\partial \dot{\gamma}}\bigg|_{\dot{\gamma}=1}, \frac{\partial F_2(\mathbf{x}; \dot{\gamma})}{\partial \dot{\gamma}}\bigg|_{\dot{\gamma}=1}\right).$$

Calculating the partial derivatives gives

$$G_1 = F_1(\theta, r),$$

and

$$G_2 = F_2(\theta, r) + \frac{1}{\alpha}(r-r_0)\left(1+\epsilon(r-r_0)^2\right).$$

We can do a reduction of our dynamical system from the varibles $(\theta, r)$ to the phase variable $\psi$ that changes along the limit cycle of the undriven system i.e. $\dot{\gamma}(t) = 1$. We now introduce this phase variable $\psi$, as is traditionally done during phase reduction of a dynamical system when analysing for synchronization [2], as follows

$$\frac{d\psi(\mathbf{x})}{dt} = \omega_n.$$

The phase variable $\psi$ is a co-ordinate along the limit cycle and it grows uniformly with $\dot{\psi} = \omega_n$ where $\omega_n = 2\pi/T_n$ with $T_n$ as the natural period of the limit cycle of the undriven system. The dynamics of this phase variable $\psi$ for the unperturbed system are given by

$$\frac{d\psi}{dt} = \omega_n = \frac{\partial\psi}{\partial\theta}\dot{\theta} + \frac{\partial\psi}{\partial r}\dot{r}$$
$$= \frac{\partial\psi}{\partial\theta}F_1(\theta, r) + \frac{\partial\psi}{\partial r}F_2(\theta, r).$$

Now, the dynamics of $\psi$ for the perturbed system can be calculated in a similar way using our leading order equations for the driven system as follows (see Chapter

7 of [2]):

$$\frac{d\psi}{dt} = \frac{\partial\psi}{\partial\theta}\dot{\theta} + \frac{\partial\psi}{\partial r}\dot{r}, \tag{3}$$
$$= \frac{\partial\psi}{\partial\theta}F_1 + \frac{\partial\psi}{\partial r}F_2 + A\left(\frac{\partial\psi}{\partial\theta}G_1 + \frac{\partial\psi}{\partial r}G_2\right)\sin(\omega t),$$
$$= \omega_n + A\left(\frac{\partial\psi}{\partial\theta}G_1 + \frac{\partial\psi}{\partial r}G_2\right)\sin(\omega t),$$
$$= \omega_n + A\,S(\psi)\sin(\omega t).$$

Note that in above, the terms on the right hand side are calculated on the limit cycle of the undriven system [2]. Here

$$S(\psi) = \frac{\partial\psi}{\partial\theta}G_1(\theta,r) + \frac{\partial\psi}{\partial r}G_2(\theta,r),$$
$$= \frac{\partial\psi}{\partial\theta}F_1(\theta,r) + \frac{\partial\psi}{\partial r}F_2(\theta,r),$$
$$+ \frac{\partial\psi}{\partial r}\frac{1}{\alpha}(r-r_0)\left(1+\epsilon(r-r_0)^2\right),$$
$$= \omega_n + S_1(\psi),$$

with

$$S_1(\psi) = \frac{\partial\psi}{\partial r}\frac{1}{\alpha}(r-r_0)\left(1+\epsilon(r-r_0)^2\right).$$

By integrating Eq. (3) for $\psi$ over one period of the driving $T = 2\pi/\omega$ we obtain

$$\int_{kT}^{(k+1)T}\frac{d\psi}{dt}dt = \int_{kT}^{(k+1)T}\omega_n dt + \int_{kT}^{(k+1)T}A\,S(\psi)\sin(\omega t)dt,$$

$$\psi_{k+1} = \psi_k + 2\pi\frac{\omega_n}{\omega} + A\,f(\psi_k), \tag{4}$$

where $f(\psi_k) = \int_{kT}^{(k+1)T} S_1(\psi)\sin(\omega t)dt$, since $\int_{kT}^{(k+1)T}\omega_n\sin(\omega t)dt = 0$. Thus, we get a circle map with some nonlinear function $f(\cdot)$ which can in general exhibit phase synchronization behaviour [3] with the quantitative details of regions of synchronization governed by the form of the nonlinearity $f(\cdot)$.

### B. Rigid particles

We now do the analysis for rigid particles. For rigid elongated particles, we only have one ODE describing the orientational dynamics as follows

$$\dot{\theta} = \frac{\dot{\gamma}}{2}\left(\frac{(r+1)^2-1}{(r+1)^2+1}\cos 2\theta - 1\right) = F(\theta;\dot{\gamma},r).$$

Here $r$ is the shape parameter and the shear rate is $\dot{\gamma} = 1 + A\sin(\omega t)$. Assuming that $A \ll 1$, we can simplify the system to the following ODE:

$$\dot{\theta} \approx F(\theta) + A\,G(\theta)\sin(\omega t),$$

where

$$G = \frac{\partial F}{\partial\dot{\gamma}}\Big|_{\dot{\gamma}=1} = F(\theta).$$

Hence we have,

$$\dot{\theta} = F(\theta) + AF(\theta)\sin(\omega t). \tag{5}$$

Introducing the phase variable $\psi$ as follows

$$\psi = \omega_n\int_0^\theta \dot{\theta}^{-1}d\theta,$$

with $\dot{\psi} = \omega_n$ where $\omega_n = 2\pi/T_n$ with $T_n$ as the period of the limit cycle of the undriven system. Thus we get,

$$\frac{d\psi}{d\theta} = \frac{\omega_n}{\dot{\theta}} = \frac{\omega_n}{F(\theta)},$$

giving

$$\frac{d\psi}{d\theta}F(\theta) = \omega_n.$$

Now the rate of change of phase variable for the driven system results in,

$$\frac{d\psi}{dt} = \frac{d\psi}{d\theta}\dot{\theta} = \frac{d\psi}{d\theta}F(\theta) + A\frac{d\psi}{d\theta}G(\theta)\sin(\omega t).$$

Here, $d\psi/d\theta$ is calculated on the limit cycle of the unperturbed system (see Chapter 7 of [2]). This gives,

$$\frac{d\psi}{dt} = \omega_n + A\frac{d\psi}{d\theta}G(\theta)\sin(\omega t). \tag{6}$$

By changing varibles everywhere from $\theta$ to $\psi$ we can rewrite the above equation as

$$\frac{d\psi}{dt} = \omega_n + A\,S(\psi)\sin(\omega t), \tag{7}$$

where $S(\psi) = \frac{d\psi}{d\theta}G(\theta)$.

Now, in general, integrating Eq. (6) over one period of the driving oscillator i.e. $T = 2\pi/\omega$ will give a Poincaré map as follows

$$\int_{kT}^{(k+1)T}\frac{d\psi}{dt}dt = \int_{kT}^{(k+1)T}\omega_n dt + A\int_{kT}^{(k+1)T}S(\psi)\sin(\omega t)dt,$$

$$\psi_{k+1} = \psi_k + 2\pi\frac{\omega_n}{\omega} + f(\psi_k), \tag{8}$$

where $f(\psi_k) = \int_{kT}^{(k+1)T}S(\psi)\sin(\omega t)dt$. This is a circle map with a nonlinear function $f(\cdot)$. Now we have

$$S(\psi) = \frac{d\psi}{d\theta}G(\theta) = \frac{d\psi}{d\theta}F(\theta) = \omega_n.$$

Hence, in this case $f(\psi_k) = 0$ and the circle map reduces to

$$\psi_{k+1} = \psi_k + 2\pi\frac{\omega_n}{\omega}.$$

This will give periodic or quasiperiodic orbits when the ratio of the two frequencies $\omega_n$ and $\omega$ is a rational or an irrational number, respectively, but it will never exhibit phase locking [3].

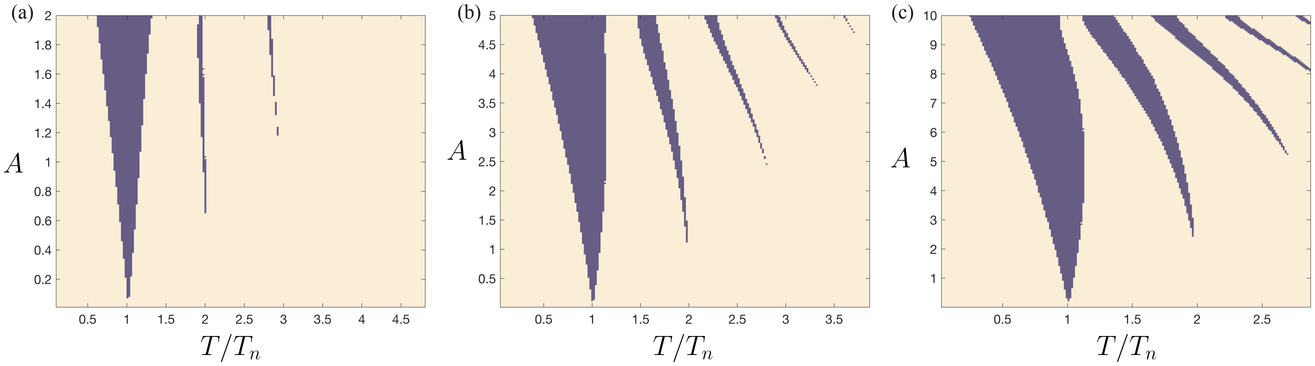


FIG. 6. Arnold tongues showing phase synchronization (violet regions) in the parameter space formed by the ratio driving period $T$ to the natural period $T_n$ and the driving amplitude $A$ for elongated particles with active shape deformations given by $r(t) = r_0 + A\sin(\omega t)$ with (a) $r_0 = 2$, (b) $r_0 = 5$ and (c) $r_0 = 10$. Here $\omega = 2\pi/T$, $\dot{\gamma} = 1$ and the natural periods are $T_n \approx 10.4$ for $r_0 = 3$, $T_n \approx 19.4$ for $r_0 = 5$, and $T_n \approx 34.8$ for $r_0 = 10$.

## III. SYNCHRONIZATION FOR ELONGATED PARTICLES WITH ACTIVE SHAPE DEFORMATIONS

In this section, we consider actively shape-changing elongated particles in steady shear flow and show that they can also exhibit phase synchronization and hence nematic order emerges for many such non-interacting particles. Motile cells and microswimmers can undergo shape fluctuations or move their appendages in a periodic way to propel themselves at low Reynolds number and these oscillatory motions maybe approximated as active shape fluctuations [4–6]. It has been shown using a triangular bead-spring model that active shape fluctuation can phase lock to flow-induced tumbling [7]. Here we analyze a simple situation of fluctuations in the shape parameter $r$ of our model. We start with the equation for orientational dynamics of the rigid elongated particle given by

$$\dot{\theta} = \frac{\dot{\gamma}}{2}\left(\frac{(r+1)^2-1}{(r+1)^2+1}\cos 2\theta - 1\right) = F(\theta; r).$$

Now, instead of varying the shear rate with time, we consider an active particle undergoing shape oscillations given by $r = r_0 + A\sin(\omega t)$ with $A \ll r_0$. Then, doing a perturbation expansion in $A$ and only keeping the leading order term we get

$$\dot{\theta} \approx F(\theta) + A\,G(\theta)\sin(\omega t),$$

where $F(\theta) = F(\theta; r)$ evaluated at $r = r_0$ and

$$G(\theta) = \frac{\partial F}{\partial r}\Big|_{r=r_0} = 2\dot{\gamma}\cos(2\theta)\frac{r_0+1}{((r_0+1)^2+1)^2}.$$

This can be written in terms of $F(\theta)$ as follows

$$G(\theta) = \frac{4(r_0+1)}{((r_0+1)^4-1)}F(\theta) + \frac{2\dot{\gamma}(r_0+1)}{((r_0+1)^4-1)}.$$

We now follow the same analysis as in Sec. II and introduce the phase variable $\psi$ giving us $\frac{d\psi}{d\theta}F(\theta) = \omega_n$ for the unperturbed system and the variations in $\psi$ for the perturbed system become

$$\begin{aligned}\frac{d\psi}{dt} &= \frac{d\psi}{d\theta}\dot{\theta} \\ &= \frac{d\psi}{d\theta}F(\theta) + A\,\frac{d\psi}{d\theta}G(\theta)\sin(\omega t) \\ &= \omega_n + A\,\frac{d\psi}{d\theta}G(\theta)\sin(\omega t).\end{aligned}$$

If we let $S(\psi) = \frac{d\psi}{d\theta}G(\theta)$ then we have,

$$\frac{d\psi}{dt} = \omega_n + AS(\psi)\sin(\omega t).$$

Integrating the above equation over one period of driving will give

$$\int_{kT}^{(k+1)T}\frac{d\psi}{dt}dt = \int_{kT}^{(k+1)T}\omega_n dt + \int_{kT}^{(k+1)T} A\,S(\psi)\sin(\omega t)dt,$$

$$\psi_{k+1} = \psi_k + 2\pi\frac{\omega_n}{\omega} + A\,f(\psi_k), \qquad (9)$$

where

$$
\begin{aligned}
f(\psi_k) &= \int_{kT}^{(k+1)T} S(\psi)\sin(\omega t)dt, \\
&= \int_{kT}^{(k+1)T} \frac{d\psi}{d\theta} G(\theta)\sin(\omega t)dt \\
&= \frac{4(r_0+1)}{((r_0+1)^4-1)}\int_{kT}^{(k+1)T} \frac{d\psi}{d\theta}F(\theta)\sin(\omega t)dt + \frac{2\dot{\gamma}(r_0+1)}{((r_0+1)^4-1)}\int_{kT}^{(k+1)T} \frac{d\psi}{d\theta}\sin(\omega t)dt \\
&= \frac{4(r_0+1)}{((r_0+1)^4-1)}\int_{kT}^{(k+1)T} \omega_n\sin(\omega t)dt + \frac{2\dot{\gamma}(r_0+1)}{((r_0+1)^4-1)}\int_{kT}^{(k+1)T} \frac{d\psi}{d\theta}\sin(\omega t)dt \\
&= \frac{2\dot{\gamma}(r_0+1)}{((r_0+1)^4-1)}\int_{kT}^{(k+1)T} \frac{d\psi}{d\theta}\sin(\omega t)dt.
\end{aligned}
$$

This again gives a circle map with some nonlinearity $f(\cdot)$ and in general the system can exhibit phase synchronization. Arnold tongues of synchronization obtained by numerically solving the system are shown in Fig. 6.

Note that we may get the form of

$$\psi(\theta) = \frac{-2\omega_0}{\sqrt{1-\beta^2}\dot{\gamma}}\arctan\left(\sqrt{\frac{1+\beta}{1-\beta}}\tan\theta\right),$$

where

$$\beta = \frac{(r_0+1)^2-1}{(r_0+1)^2+1}.$$

This allows us to explicitly calculate $d\psi/d\theta$ in terms of $\psi = \omega_0 t$ and hence get the functional form of the circle map.

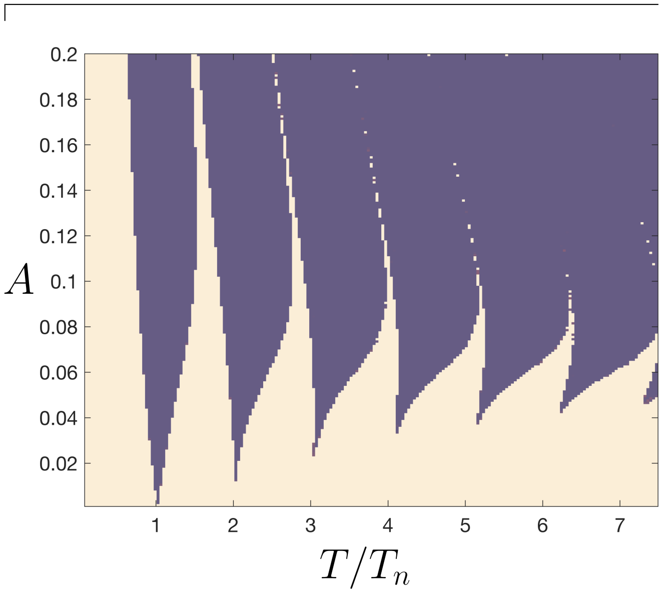


FIG. 7. Arnold tongues showing phase synchronization (violet regions) in the parameter space formed by the ratio of the driving period $T$ to the natural period $T_n$ and the driving amplitude $A$ for rigid elongated particles with fluctuating chirality given by $\omega_a(t) = A\sin(\omega t)$ with $r_0 = 3$. Here $\omega = 2\pi/T$, $\dot{\gamma} = 1$ and $T_n \approx 13.35$.

## IV. SYNCHRONIZATION FOR RIGID ELONGATED PARTICLES WITH OSCILLATING CHIRAL ACTIVITY

In addition to shape oscillations, periodic driving of other internal degrees of freedom may also result in phase-synchronized nematic order. We consider rigid nematic particles in steady shear flow having a time-periodic internal chiral activity. The orientational dynamics of such a particle is given by

$$\dot{\theta} = \frac{\dot{\gamma}}{2}\left(\frac{(r+1)^2-1}{(r+1)^2+1}\cos(2\theta)-1\right) + \omega_a(t) \qquad (10)$$

where $\omega_a(t) = A\sin(\omega t)$ is a pulsating internal chiral activity i.e. angular velocity and the other parameters are fixed and same as before. We can rewrite our system in the form

$$\dot{\theta} = F(\theta) + A\,G(\theta)\sin(\omega t),$$

where

$$F(\theta) = \frac{\dot{\gamma}}{2}\left(\frac{(r+1)^2-1}{(r+1)^2+1}\cos(2\theta)-1\right),$$

and $G(\theta) = 1$. We now follow the same analysis as in Sec. II and introduce the phase variable $\psi$ as follows

$$\psi = \omega_n \int_0^\theta \dot{\theta}^{-1} d\theta,$$

giving us $\frac{d\psi}{d\theta}F(\theta) = \omega_n$ for the unperturbed system and the variations in $\psi$ for the perturbed system become

$$
\begin{aligned}
\frac{d\psi}{dt} &= \frac{d\psi}{d\theta}\dot{\theta} \\
&= \frac{d\psi}{d\theta}F(\theta) + A\frac{d\psi}{d\theta}G(\theta)\sin(\omega t) \\
&= \omega_n + A\frac{d\psi}{d\theta}\sin(\omega t).
\end{aligned}
$$

If we let $S(\psi) = \frac{d\psi}{d\theta}$ then we have,

$$\frac{d\psi}{dt} = \omega_n + AS(\psi)\sin(\omega t).$$

Integrating the above equation over one period of driving will give

$$\int_{kT}^{(k+1)T} \frac{d\psi}{dt} dt = \int_{kT}^{(k+1)T} \omega_n dt + \int_{kT}^{(k+1)T} A\, S(\psi)\sin(\omega t) dt,$$

$$\psi_{k+1} = \psi_k + 2\pi \frac{\omega_n}{\omega} + f(\psi_k), \tag{11}$$

where $f(\psi_k) = \int_{kT}^{(k+1)T} \frac{d\psi}{d\theta} \sin(\omega t) dt$. This again gives a circle map with some nonlinearity $f(\cdot)$ and in general the system can exhibit phase synchronization. Arnold tongues of synchronization obtained by numerically solving the system are shown in Fig. 7.

## V. PHASE SYNCHRONIZATION IN A CONTINUUM MODEL OF DEFORMABLE NEMATIC PARTICLES

Our results presented in the main text can also be extended to a dense suspension of nematic particles. A dense suspension of deformable, nematic particles is described by the continuum theory of nematohydrodynamics equations [8]. In a one-dimensional channel setup (along the $y$ co-ordinate) with simple shear flow having shear rate $\dot{\gamma}$; the equations of motion reduce to the following:

$$\begin{aligned}
\dot{\theta} &= \frac{\dot{\gamma}}{2}\left(\lambda_0 \frac{(r+1)^2 - 1}{(r+1)^2 + 1}\cos 2\theta - 1\right) \\
&\quad + \Gamma_\theta K_0 \frac{\partial}{\partial y}\left[\left(\frac{r}{1+r}\right)^2 \frac{\partial \theta}{\partial y}\right], \\
\dot{r} &= \dot{\gamma}(r+1)\sin 2\theta - \Gamma_r A_r (r - r_0)\left(1 + \epsilon (r - r_0)^2\right) \\
&\quad - \Gamma_r K_0 \frac{r}{(1+r)^3}\left(\frac{\partial \theta}{\partial y}\right)^2 .
\end{aligned} \tag{12}$$

Here $r$ and $\theta$ represent averaged quantities i.e. averaged shape deformation and average orientation, respectively, of a collection of deformable nematic particles in some localized region. The parameter $\lambda_0$ is a flow aligning scale determining the effects of fluid flow on the dense suspension, and the parameter $K_0$ is an elastic constant penalizing gradients in nematic orientation. The dynamical system in Eq. (12) result in nematic order due to the terms $\propto K_0$ which smooth out variations in the nematic orientation. These terms capture the effects of microscopic interactions between nematic particles. If we allow the shear rate to be time-dependent in this continuum model i.e. $\dot{\gamma}(t)$, then one obtains different behaviors depending on $K_0$. For high temperatures when the system is in an isotropic state, $K_0$ is very small, the Eq. (12) are same as that for individual particles in the main text with the extra parameter $\lambda_0$. Hence, all our results for phase-synchronization still hold in this limit. In fact, in the case where $\lambda_0 > 1$ synchronization is enhanced as it exacerbates the critical slowing down in the ghost region. This is because the saddle-node infinite period (SNIPER) bifurcation of the limit cycle, that takes place at $r \to \infty$ for individual particles, occurs for finite $r$ value in continuum model. In the regime where the nematic elasticity $K_0$ is large (system without shear flow has orientational order), the system encounters two effects simultaneously - the time-dependent shear driving force trying to synchronize the particles through the phase synchronization mechanism and the nematic elasticity $K_0$ trying to smooth out orientational order of the particles.

## SUPPLEMENTAL VIDEOS

**Supplemental Video S1:** Video showing phase synchronization and the corresponding emergence of nematic order for non-interacting deformable particles in an oscillatory shear flow corresponding to Fig. 1(c) of the main text.

**Supplemental Video S2:** Video showing that nematic order does not emerge for non-interacting rigid particles in an oscillatory shear flow corresponding to Fig. 1(d) of the main text.

**Supplemental Video S3:** Video showing that nematic order does not emerge for non-interacting deformable particles in a shear flow (with $A = 0$) corresponding to Fig. 2(c) of the main text.

**Supplemental Video S4:** Video showing phase synchronization and the corresponding emergence of nematic order for non-interacting deformable particles in an oscillatory shear flow (with $A > 1$) corresponding to Fig. 4 of the Supplemental Material.

**Supplemental Video S5:** Video showing phase synchronization and the corresponding emergence of nematic order for non-interacting deformable particles in an oscillatory shear flow (with no mean shear flow component) corresponding to Fig. 5 of the Supplemental Material.

[1] A. Pikovsky, M. Rosenblum, and J. Kurths, Phase synchronization in regular and chaotic systems, International Journal of Bifurcation and Chaos **10**, 2291 (2000).

[2] A. Pikovsky, M. Rosenblum, and J. Kurths, *Synchronization: A Universal Concept in Nonlinear Sciences*, Cambridge Nonlinear Science Series (Cambridge University

Press, 2001).
[3] E. A. Jackson, Models based on first order difference equations, in *Perspectives of Nonlinear Dynamics* (Cambridge University Press, 1989) p. 142–225.
[4] R. Ma, G. S. Klindt, I. H. Riedel-Kruse, F. Jülicher, and B. M. Friedrich, Active phase and amplitude fluctuations of flagellar beating, Phys. Rev. Lett. **113**, 048101 (2014).
[5] A. Taloni, E. Kardash, O. U. Salman, L. Truskinovsky, S. Zapperi, and C. A. M. La Porta, Volume changes during active shape fluctuations in cells, Phys. Rev. Lett. **114**, 208101 (2015).
[6] W. D. Piñeros and E. Fodor, Biased ensembles of pulsating active matter, Phys. Rev. Lett. **134**, 038301 (2025).
[7] M. S. Rizvi, A. Nait-Ouhra, A. Farutin, P. Peyla, S. Rafai, and C. Misbah, Rheological signature of microswimmer phase-locking under flow, Phys. Rev. Fluids **4**, 103302 (2019).
[8] I. Hadjifrangiskou, L. J. Ruske, and J. M. Yeomans, Active nematics with deformable particles, Soft Matter **19**, 6664 (2023).
